# Supplementary material for: Boosting in Image Quality Assessment
Source: arXiv:1811.08429 ancillary file (2018-11-21)
Supplement: Supplementary file 1 [file slides.pdf]

# Boosting in Image Quality Assessment

**Can Temel\* and Ghassan AlRegib**

**Multimedia and Sensors Lab (MSL)  
Center for Signal and Information Processing (CSIP)  
Georgia Institute of Technology  
September 21, 2016**

# Outline

## I. Introduction

- Image Quality Assessment
- Boosting

## II. Experimental Setup

- Image Quality Estimators
- Boosting Methods and Test Setup

## III. Experimental Analysis

- Performance Comparison of Existing, Regressed, and Boosted Methods
- Boosting Performance with respect to Number of Fused Methods

## IV. Conclusion

# I. Introduction

## Image Quality Assessment: Why?

### Remote assistance

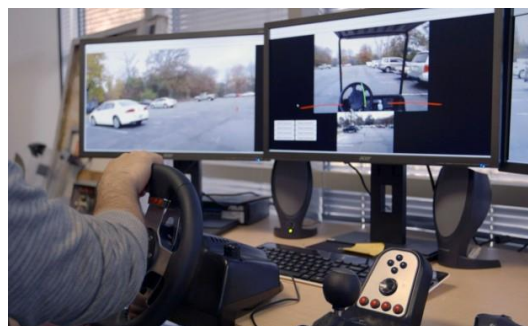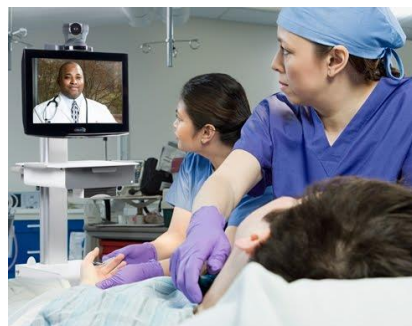

### Smart capturing

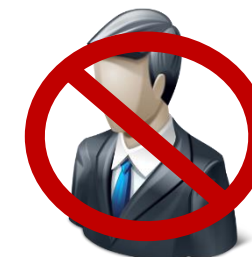

| Application                                                                       | Average daily shared photos <sup>[1]</sup> |
|-----------------------------------------------------------------------------------|--------------------------------------------|
| 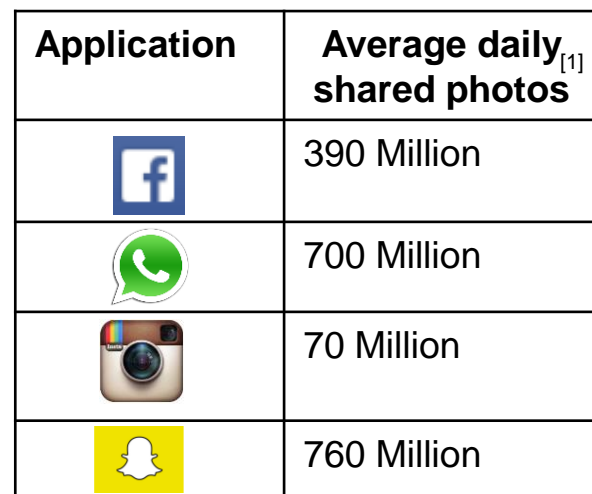 | 390 Million                                |
| 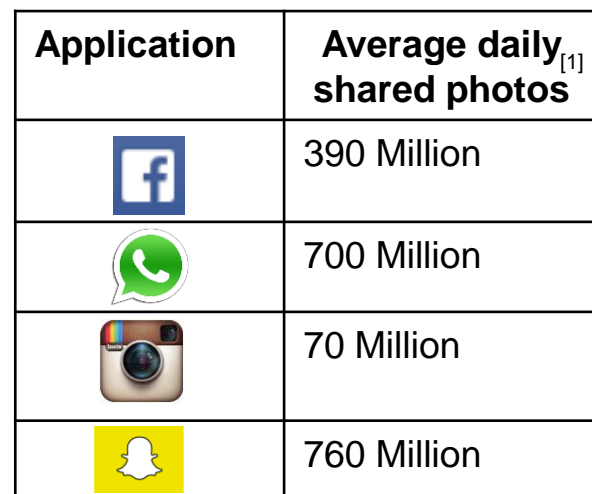 | 700 Million                                |
| 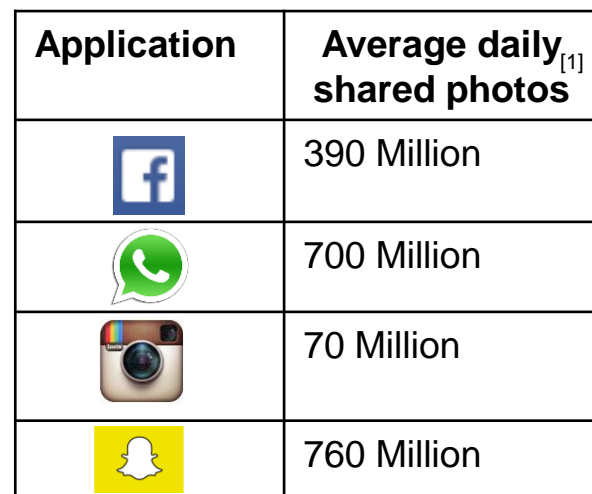 | 70 Million                                 |
| 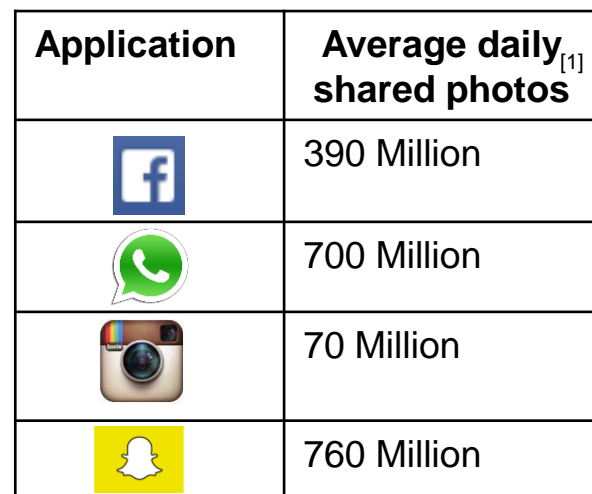 | 760 Million                                |

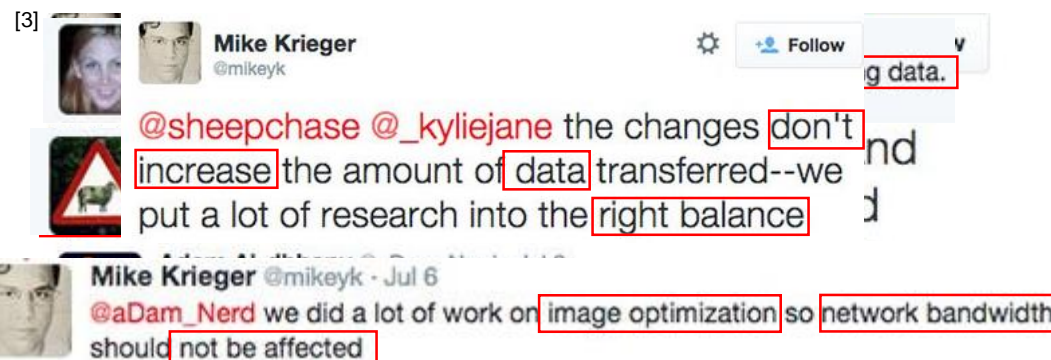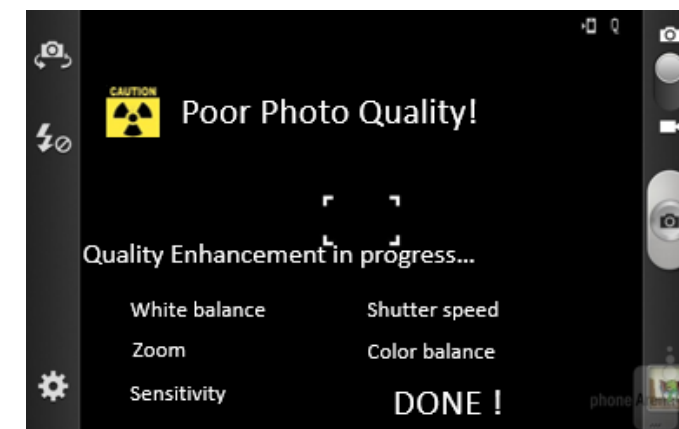

[1] Adweek, <http://www.adweek.com/socialtimes/how-many-photos-are-uploaded-to-snapchat-every-second/621488>, Jun 2015

[2] LG, "Ultra Clarity, Ultra Scale," [http://www.lg.com/levant\\_en/Mini-page-ultra/index](http://www.lg.com/levant_en/Mini-page-ultra/index)

[3] PetPixel, <http://petapixel.com/2015/07/08/instagram-resolution-increase-heres-how-it-affects-image-quality-and-file-size/>, July 8, 2015

# I. Introduction

## Image Quality Assessment: How?

Test setup

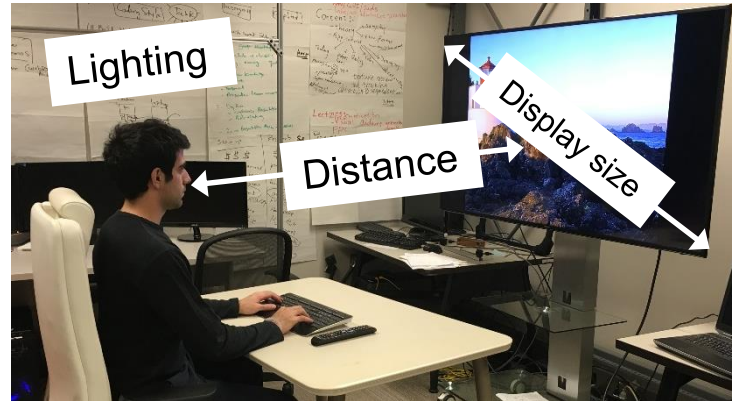

Reference images [1]

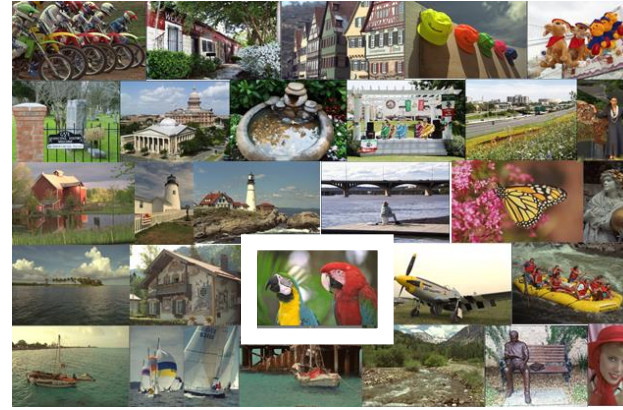

Distorted images [1]

Subjective Scores

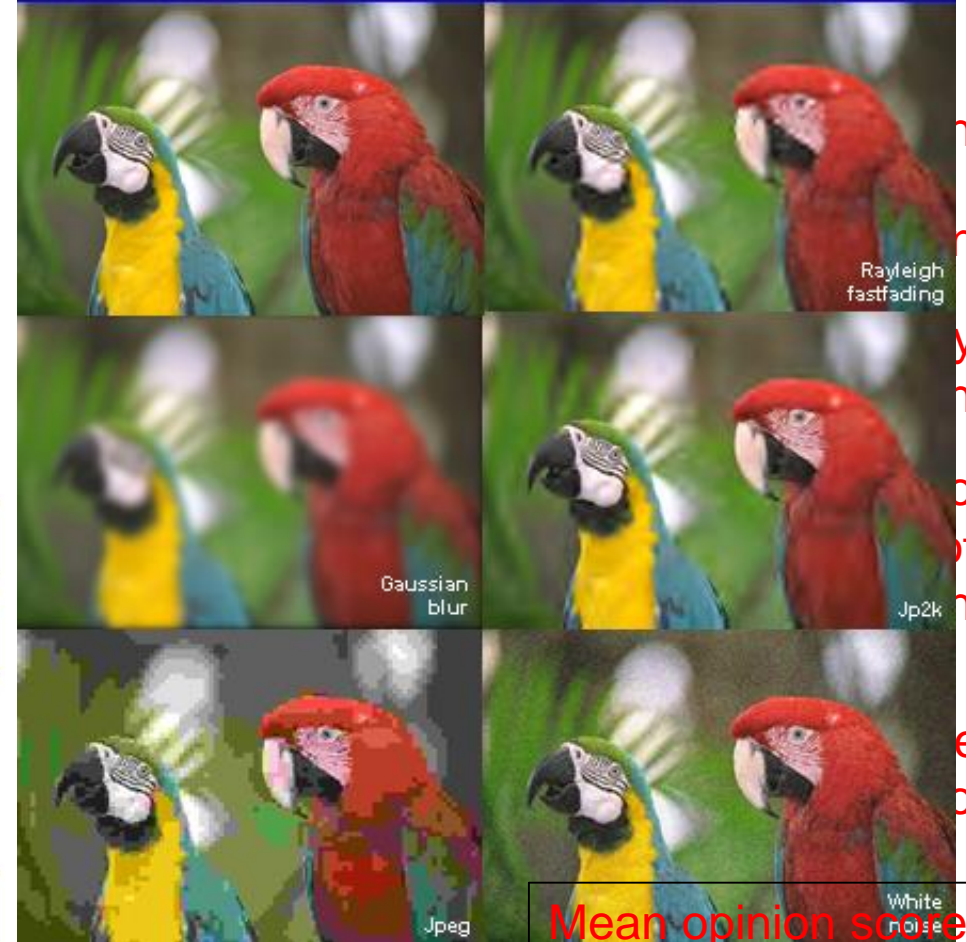

P2P pipeline

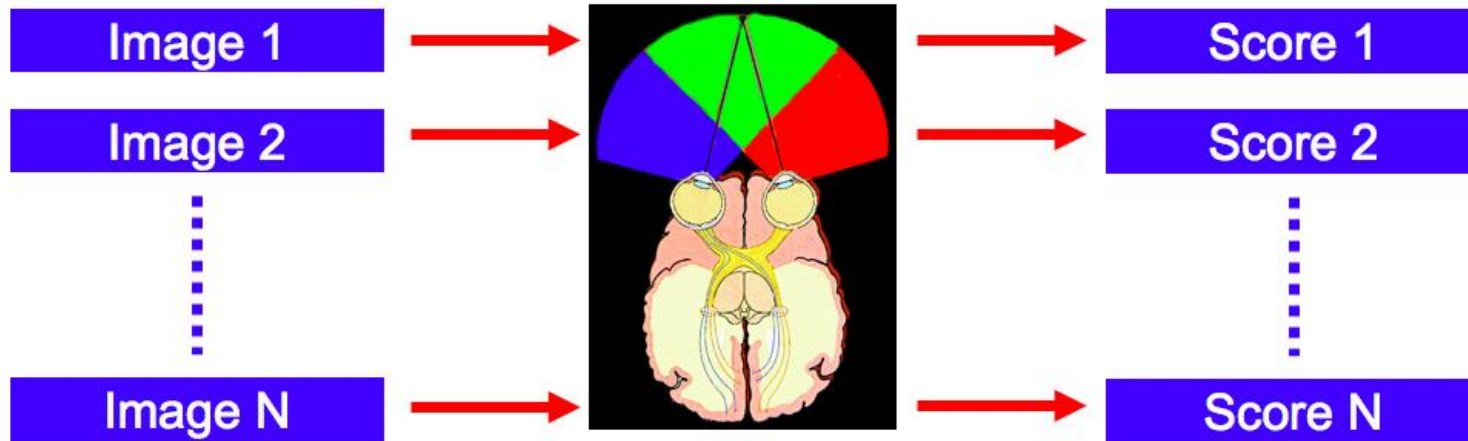

[1] Sheikh, H.R., Wang, Z., Cormack, L. and Bovik, A.C., "LIVE Image Quality Assessment Database Release 2", <http://live.ece.utexas.edu/research/quality>.



# I. Introduction

## Image Quality Assessment: How?

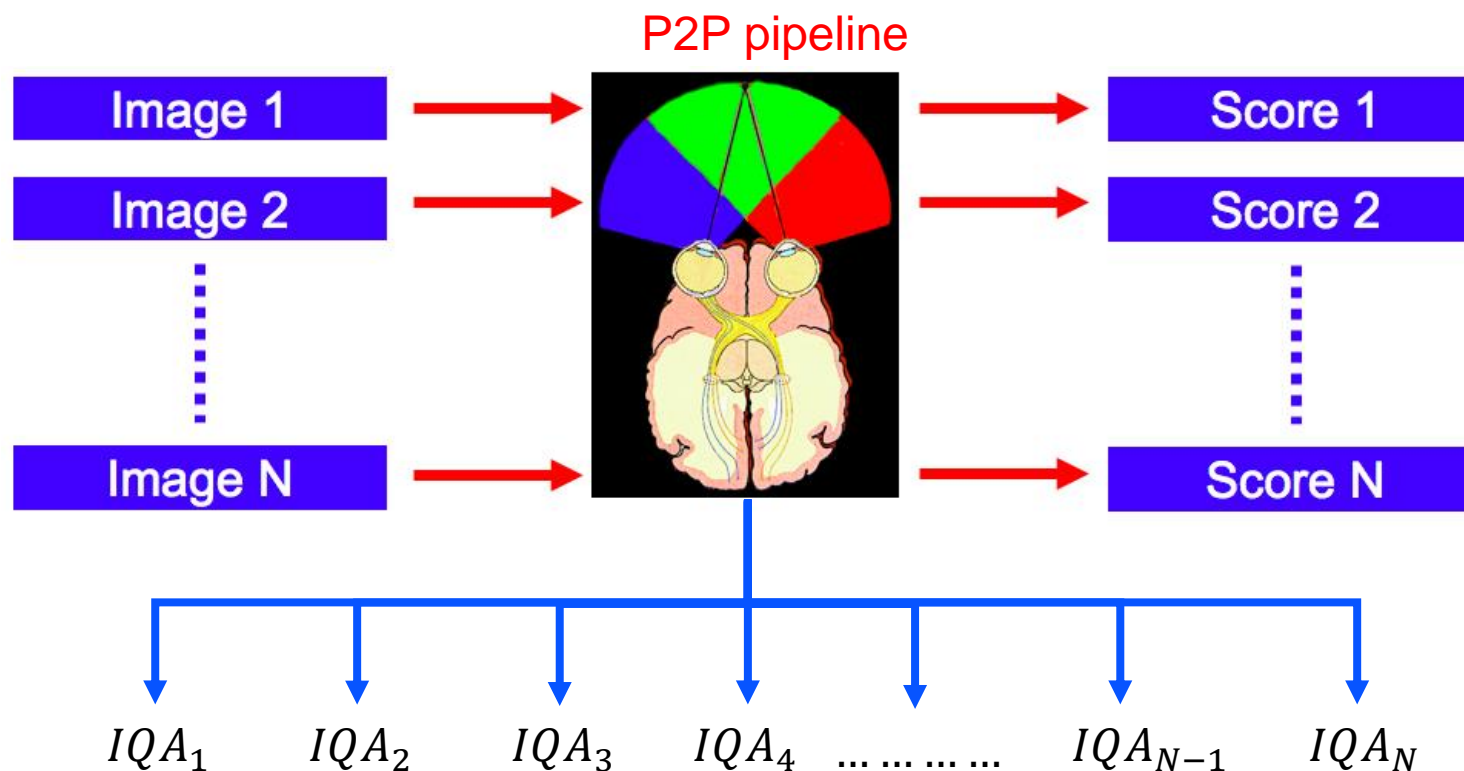

Is it possible to obtain **strong** learners from **weak learners**?

*Kearns, 1988*

*Kearns and Valiant, 1994*

# I. Introduction

## Boosting

| YEAR               |        | 2008                                 | 2011              | 2013 | 2015 |
|--------------------|--------|--------------------------------------|-------------------|------|------|
| QUALITY ESTIMATORS |        | <i>Liu and Yang</i>                  | <i>Liu et al.</i> |      |      |
| Fidelity           |        |                                      |                   |      |      |
| Structure          |        |                                      |                   |      |      |
| Scale Space        |        |                                      |                   |      |      |
| Visual system      |        |                                      |                   |      |      |
| Color              |        |                                      |                   |      |      |
| Boosting Method    | SVR    |                                      |                   |      |      |
|                    | Others | Canonical<br>Correlation<br>Analysis |                   |      |      |

### *Generalizability*

- Boosting > regression ?
- Boosting performance (number of fused methods) ?

### *Superiority*

- An alternative approach >SVR ?

# II. Experimental Setup

## Boosting Methods and Test Setup

### Boosting Methods

Support Vector Machines  
(SVM)

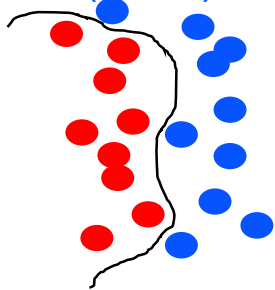

Neural Networks  
(NN)

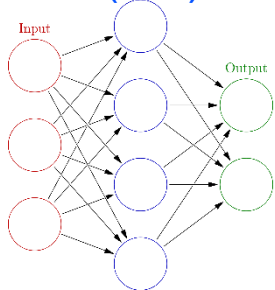

### Databases

|               | LIVE | MULTI | TID13 | Total |
|---------------|------|-------|-------|-------|
| Compression   | 460  | 180   | 375   | 1015  |
| Image Noise   | 174  | 180   | 1375  | 1729  |
| Communication | 174  | -     | 250   | 424   |
| Blur          | 174  | 315   | 250   | 739   |
| Color         | -    | -     | 375   | 375   |
| Global        | -    | -     | 250   | 250   |
| Local         | -    | -     | 250   | 250   |

### Performance Metrics

RMSE

$$\sqrt{E[X - Y]^2}$$

Pearson  
Correlation

$$\frac{E[(X - \mu_X)(Y - \mu_Y)]}{\sigma_X \sigma_Y}$$

Spearman  
Correlation

$X_i, Y_i \longrightarrow x_i, y_i$

$$1 - \frac{6 \sum_{i=1}^N (x_i - y_i)^2}{N(N^2 - 1)}$$

# II. Experimental Setup

## Image Quality Estimators

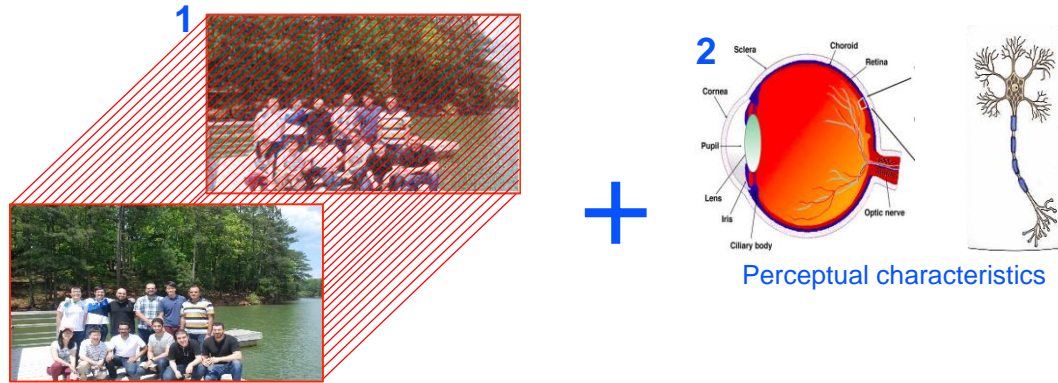

1. Fidelity: *MSE, PSNR*
2. Perceptually-extended fidelity: *PSNR-HA, PSNR-HMA*
3. Structure: *SSIM, MS-SSIM, CW-SSIM, IW-SSIM, SR-SIM (Spectral)*
4. Color: *FSIMc, PerSIM*
5. Learning: *UNIQUE*

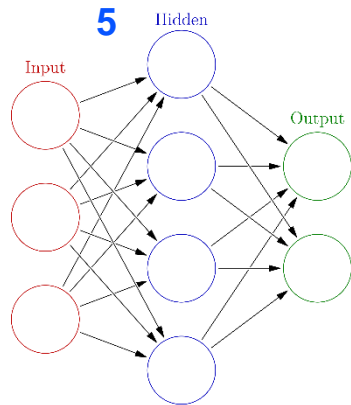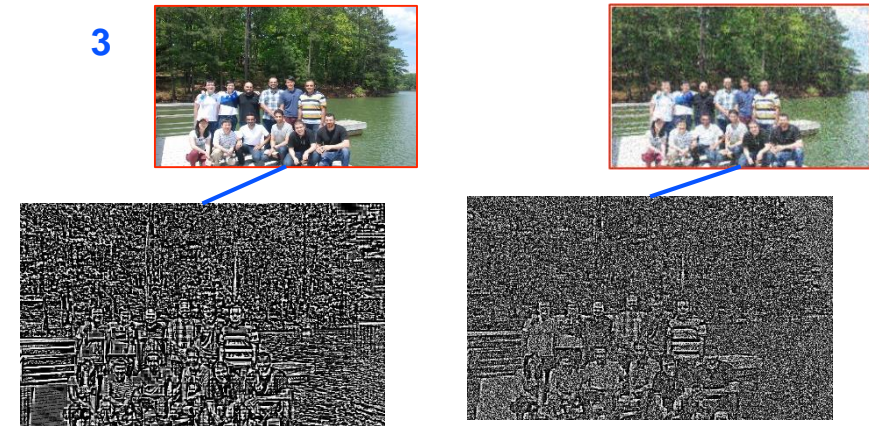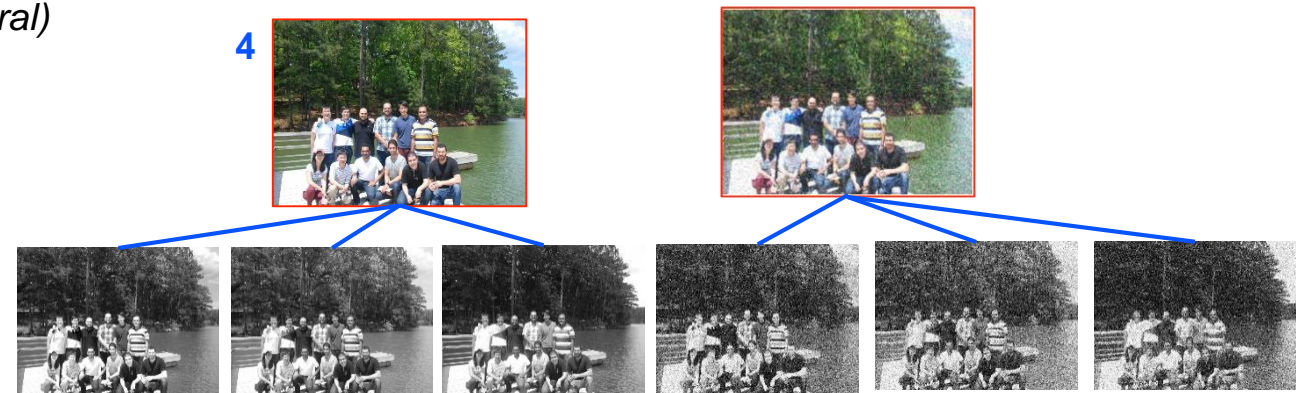



# III. Experiments

## Part I: Performance comparison of existing, regressed, and boosted quality estimators

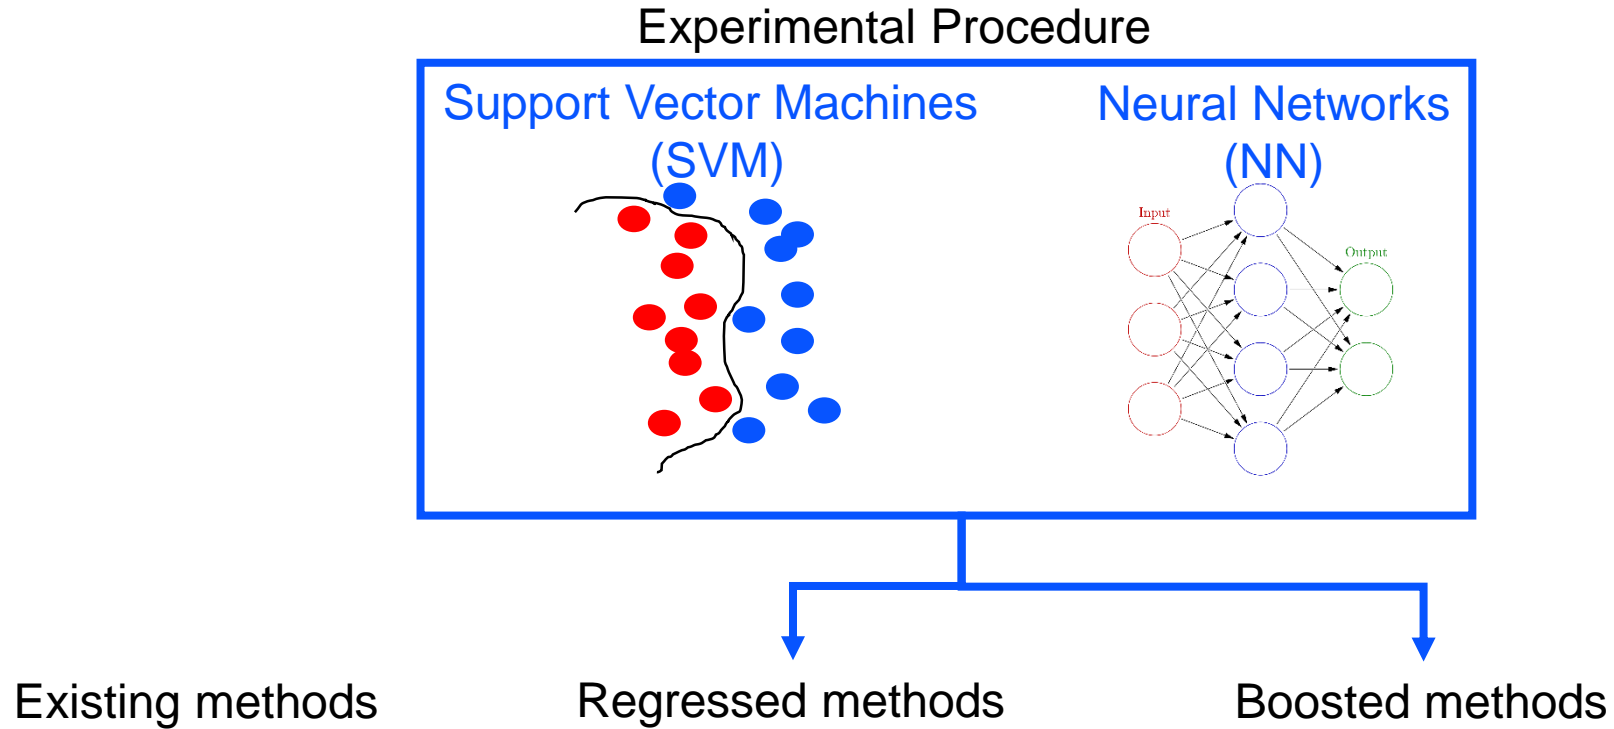

# III. Experiments

## Part I: Performance comparison of existing, regressed, and boosted quality estimators

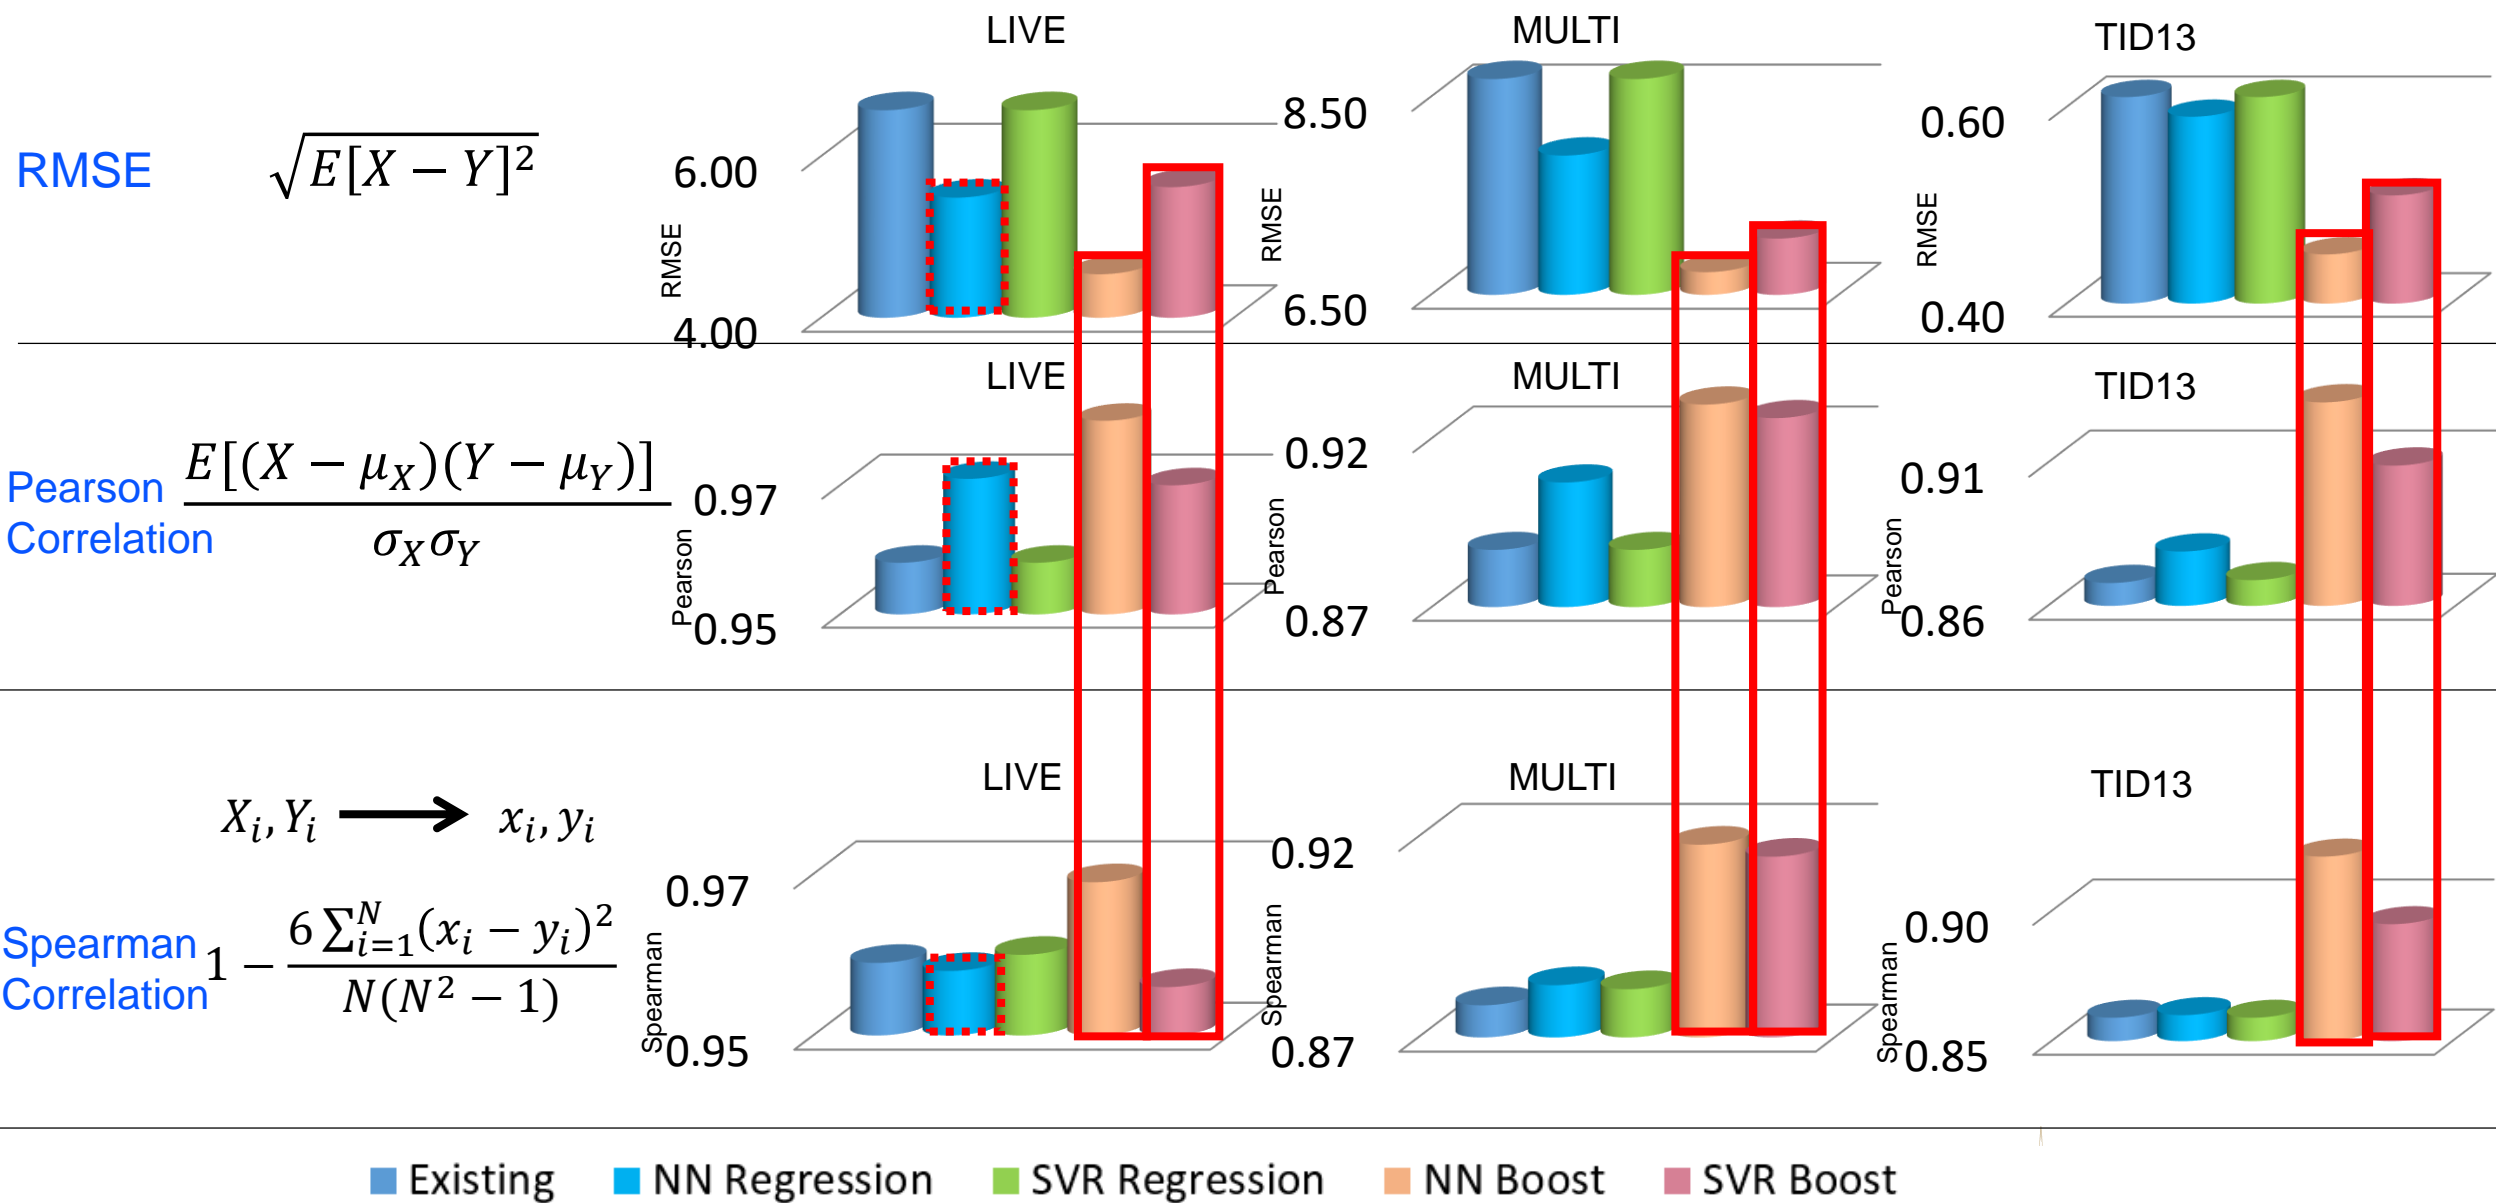

# III. Experiments

## Part I: Performance comparison of existing, regressed, and boosted quality estimators

### Generalizability

- Boosting > regression?

### Superiority

- An alternative approach >SVR ?

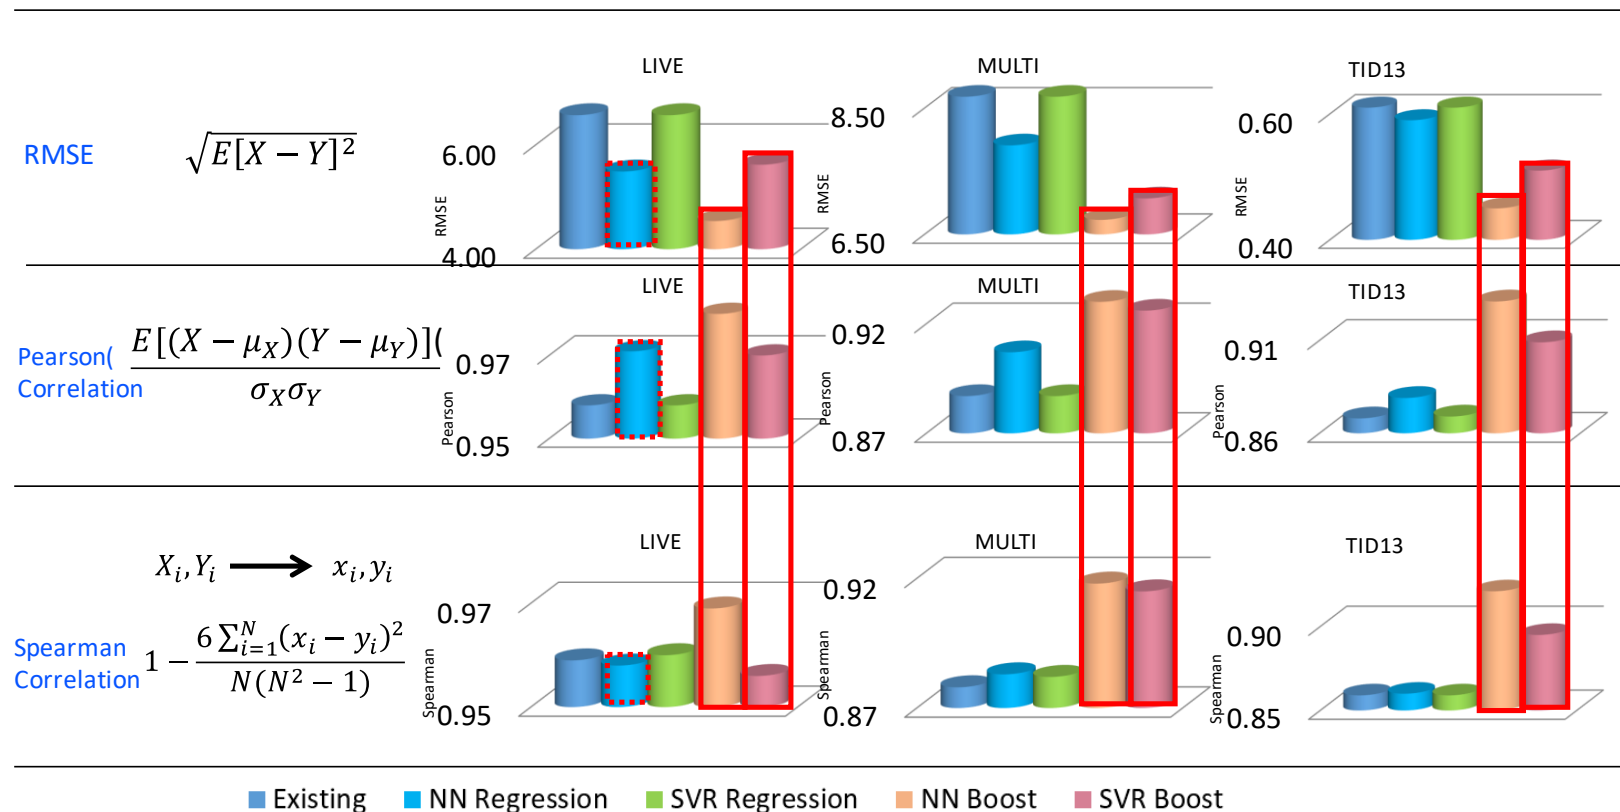

# III. Experiments

## Part II: Boosting Performance with respect to Number of Fused Methods

### Experimental Procedure

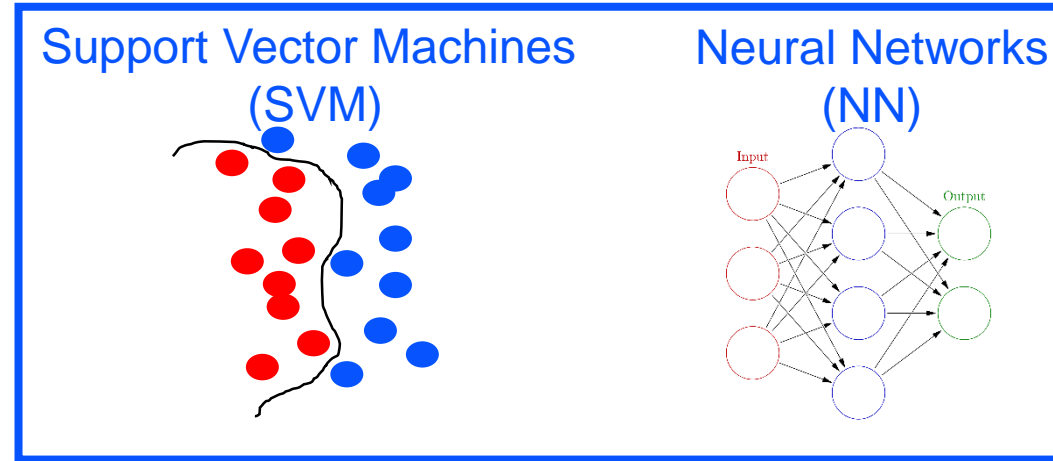

**Sort** existing methods with respect to their **performance** from the worst to the best.

**Regress** the **worst** performing method (with respect to each performance metric).

**Boost** with the **next best** performing method until all the methods are utilized.



# III. Experiments

## Part II: Boosting Performance versus Number of Fused Methods

RMSE

$$\sqrt{E[X - Y]^2}$$

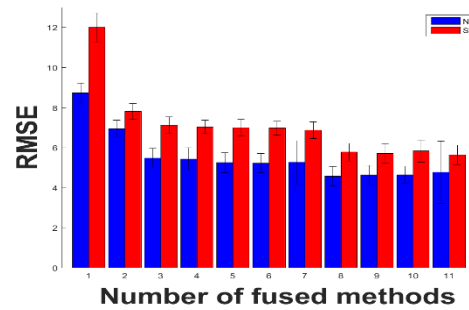

LIVE

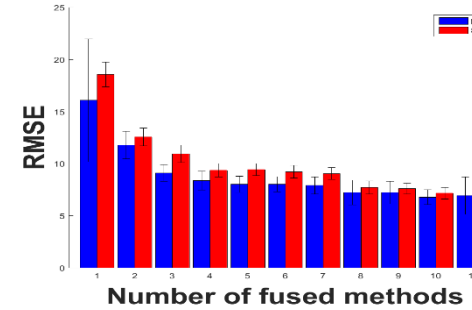

MULTI

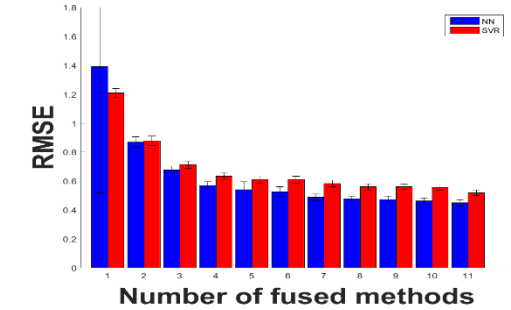

TID13

Pearson  
Correlation

$$\frac{E[(X - \mu_X)(Y - \mu_Y)]}{\sigma_X \sigma_Y}$$

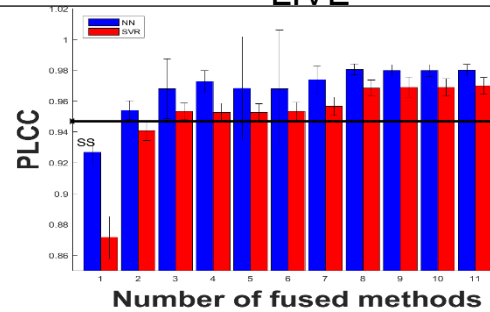

LIVE

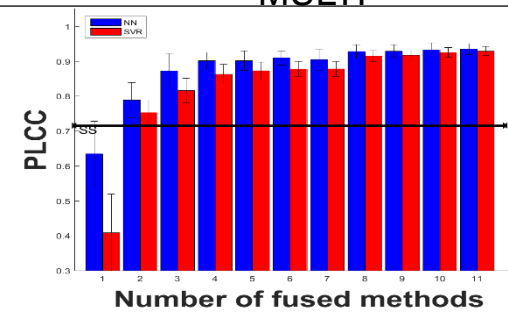

MULTI

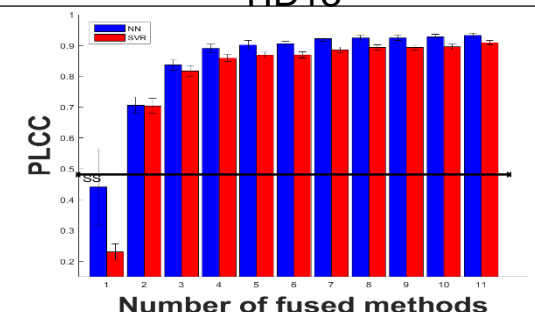

TID13

Spearman  
Correlation

$$X_i, Y_i \longrightarrow x_i, y_i$$

$$1 - \frac{6 \sum_{i=1}^N (x_i - y_i)^2}{N(N^2 - 1)}$$

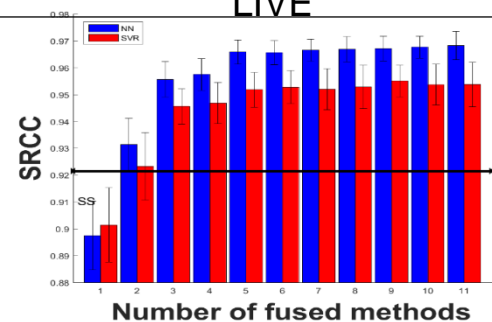

LIVE

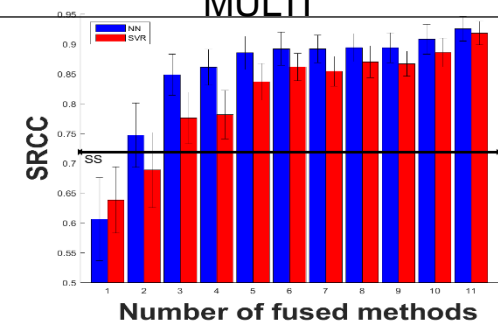

MULTI

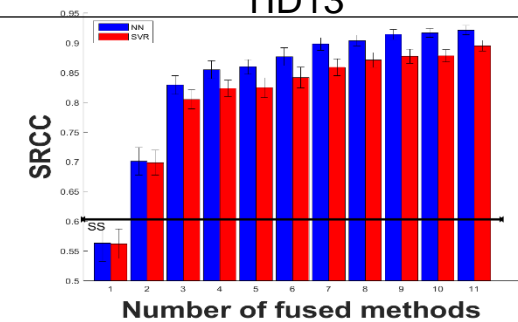

TID13

# III. Experiments

## Part II: Boosting Performance with respect to Number of Fused Methods

### Generalizability

- Boosting performance (number of fused methods) ?

### Superiority

- An alternative approach >SVR ?

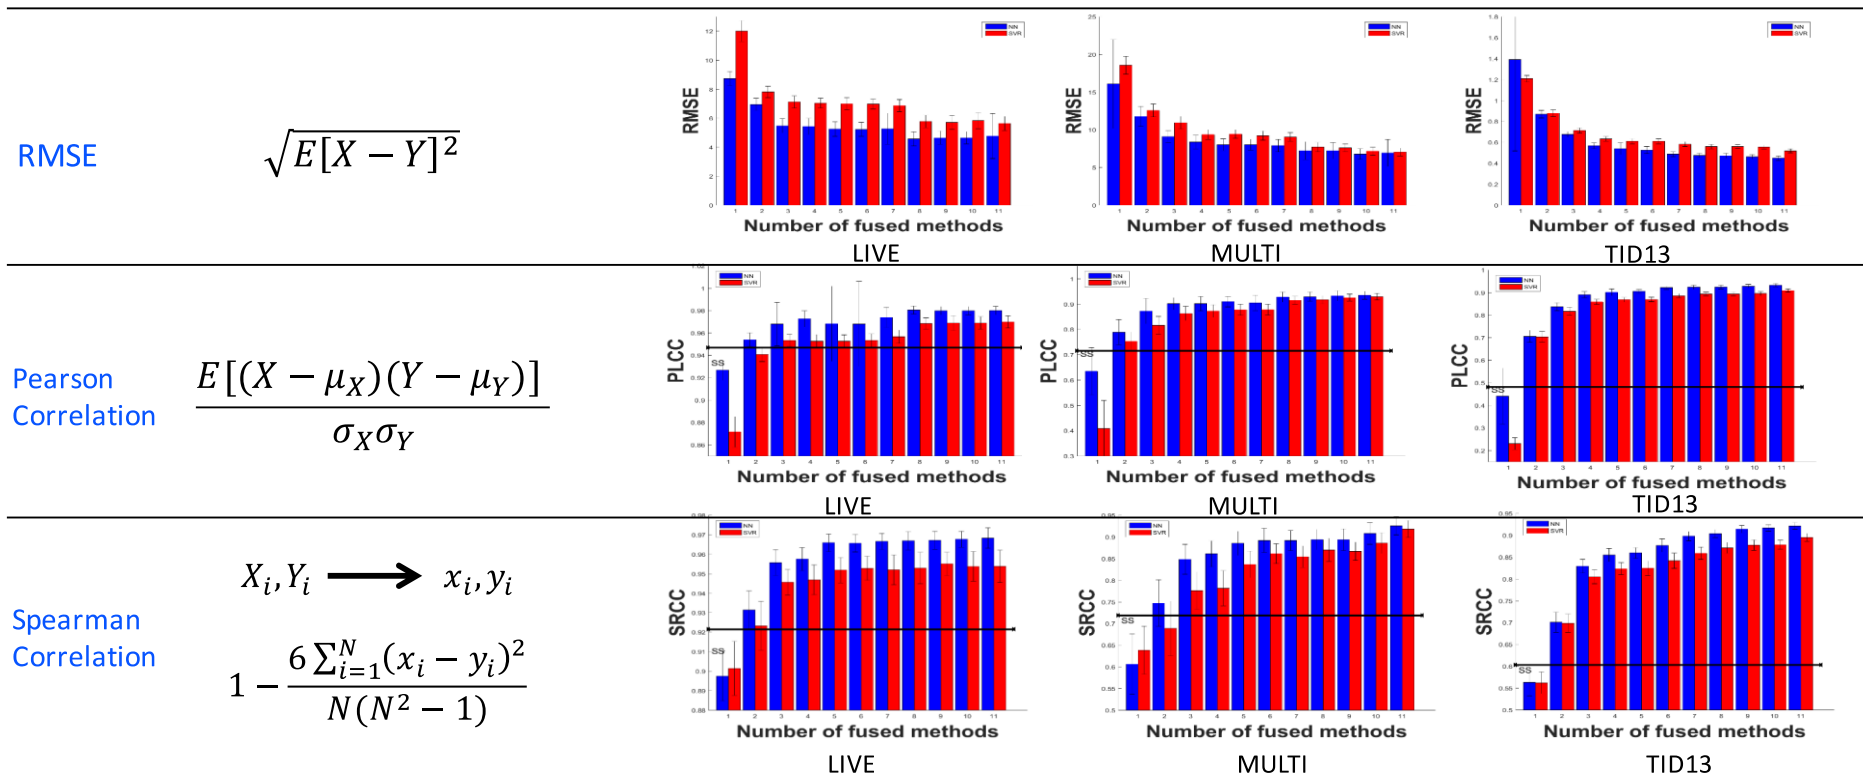

## IV. Conclusion Findings

| YEAR               |        | 2008                           | 2011 | 2013 | 2015 | 2016           |
|--------------------|--------|--------------------------------|------|------|------|----------------|
| QUALITY ESTIMATORS |        | Liu                            |      |      |      | Temel          |
| Fidelity           |        |                                |      |      |      |                |
| Structure          |        |                                |      |      |      |                |
| Scale Space        |        |                                |      |      |      |                |
| Visual system      |        |                                |      |      |      |                |
| Color              |        |                                |      |      |      |                |
| Boosting Method    | SVR    |                                |      |      |      |                |
|                    | Others | Canonical Correlation Analysis |      |      |      | Neural Network |

- **Boosting**-based methods generally **outperform existing** best performing methods.
- **Boosting** the **worst** performing quality estimator with two or more additional methods leads to statistically **significant improvements** in all the test scenarios (independent of the boosting technique).
- Boosting-based performance enhancement **level** depends on the **type** of the boosting **strategy**.
- **Neural network**-based boosting outperforms **support vector machine**-based boosting (when two or more methods are fused).

# IV. Conclusion

## Prospective Research Directions

- The **complexity** of the estimators can be considered while boosting.
- The **relationship** between the characteristics of quality estimators and the distortion types can be analyzed through boosting.
- Instead of boosting final scores, **feature maps** can be boosted to obtain hybrid methods.
- **Deep** architectures can be used for boosting feature maps.
